# Supplementary material for: Autodetachment of diatomic carbon anions from long-lived high-rotation quartet states
Source: arXiv:2405.06514 source file (2024-09-17)
Supplement: Supplementary file 1 [file suppl.pdf]

## Supplementary online information

This is a supplementary material to the paper "Autodetachment of diatomic carbon anions from long-lived high-rotation quartet states" by V. C. Schmidt *et al.* This material consists of two sections. In the first section we derive the form of the complex nonlocal operator $F(E)$ for the case of the final $\Pi_u$ states of the neutral molecule. The second section discusses a simplified form of this operator in a local approximation. The imaginary part of the level-shift operator $F(E)$ is expressed in terms of the partial widths $\Gamma_l$ that are extracted from ab-initio $R$-matrix calculations.

### I. NONLOCAL LEVEL-SHIFT OPERATOR $F(E)$ FOR THE NEUTRAL $\Pi$ STATES

In the nonlocal resonance model, the effective Hamiltonian that drives the decaying nuclear wave function of the negative ion can be written as [1]

$$H_{\text{eff}} = T + \frac{N(N+1)}{2\mu R^2} + V_d(R) + F(E) \ , \tag{1}$$

where the first two terms describe the rovibrational kinetic energy, $V_d(R)$ is the discrete-state potential curve, and $F(E)$ denotes the complex-valued level-shift operator that contains all the couplings between the resonant and continuum states of the anion in a form of a nonlocal complex-valued interaction.

The modification of the interaction operator $F(E)$, for our particular case, follows the ideas presented in Ref. [2]. The necessary differences arise from the intrinsic coupling of the degenerated electronic non-$\Sigma$ states with the molecular rotations [3]. Therefore, the neutral target electronic state $w(\tau)$ will also enter the derivation. The symbol $\tau$ here represents, collectively, the space coordinates of the target electrons. Note that the anion state is still considered to be in the $\Lambda = 0$ state, presently the $\mathrm{C}^4\Sigma_u^+$ state of $\mathrm{C}_2^-$. We start from the definition of the $F(E)$ by T.F. O'Malley [4]

$$F(E) = \langle d|QHPG_pPHQ|d\rangle \ , \tag{2}$$

where $Q$ and $P$ are the projection operators [4, 5], $G_p = 1/P(E - H + i\epsilon)P$, the discrete state of the anion is represented by $|d\rangle$, and the total Hamiltonian can be written as a sum of the nuclear kinetic energy $T$ and of the electronic Hamiltonian $H_{\text{el}}$, i.e. $H = T + H_{\text{el}}$. The projection operator $P$ can be expressed in the adiabatic energy-normalized eigenstates $|\boldsymbol{k}^{(+)}\rangle$ of the $PH_{\text{el}}P$ operator as [2]

$$P = \int d\boldsymbol{k}\, |\boldsymbol{k}^{(+)}\rangle\langle \boldsymbol{k}^{(+)}| \ . \tag{3}$$

After inserting the expansion (3) into Eq. (2) we can write

$$F(E) = \int d\boldsymbol{k}d\boldsymbol{q}\, \langle d|H_{\text{el}}|\boldsymbol{k}^{(+)}\rangle\langle \boldsymbol{k}^{(+)}|G_p|\boldsymbol{q}^{(+)}\rangle\langle \boldsymbol{q}^{(+)}|H_{\text{el}}|d\rangle \ . \tag{4}$$

The anion's background states $|\boldsymbol{k}^{(+)}\rangle$ are first written in the body frame coordinates $\boldsymbol{r}'$ and $\tau$

$$\langle \boldsymbol{r}'|\boldsymbol{k}'^{(+)}\rangle = \frac{1}{\sqrt{2}}\mathcal{A}\sum_{ll'}\frac{1}{r'}\left[w_\Lambda(\tau)\phi_{ll'}^{-\Lambda}(k,r')Y_{l-\Lambda}(\hat{\boldsymbol{r}}')Y^*_{l'-\Lambda}(\hat{\boldsymbol{k}}') + \eta w_{-\Lambda}(\tau)\phi_{ll'}^{\Lambda}(k,r')Y_{l\Lambda}(\hat{\boldsymbol{r}}')Y^*_{l'\Lambda}(\hat{\boldsymbol{k}}')\right] \ , \tag{5}$$

where the symbol $\mathcal{A}$ antisymmetrizes the wave function with respect to the exchange of the anion's electronic coordinates. Quantum number $\eta$ denotes the parity of the anion state with respect to the reflection on the body-frame coordinate plane $(x'z')$, that changes $w_\Lambda$ into $(-1)^\Lambda w_{-\Lambda}$ [6]. Recall that $w_\Lambda$ and $w_{-\Lambda}$ are different but degenerate for $\Lambda \neq 0$. For simplicity, the anionic wave function in the above equation is already assumed to possess the $\Sigma_u^+$ symmetry as the neutral target state $w_\Lambda$ couples only with the continuum wave function with the $-\Lambda$ projection of its angular momentum $l$ onto the molecular axis.

The matrix elements

$$V_{d\boldsymbol{k}} = \langle d|H_{\rm el}|\boldsymbol{k}'^{(+)}\rangle \tag{6}$$

in Eq. (4) are first written in the body frame of reference as

$$V_{d\boldsymbol{k}'} = \frac{1}{\sqrt{2}}\sum_{l'}\left[V_{dkl'}^{-\Lambda}Y_{l'-\Lambda}^*(\hat{\boldsymbol{k}}') + \eta V_{dkl'}^{\Lambda}Y_{l'\Lambda}^*(\hat{\boldsymbol{k}}')\right] , \tag{7}$$

with

$$V_{dkl'}^{\Lambda} = \sum_{l}\langle d|H_{\rm el}|\mathcal{A}\,\frac{1}{r}\,w_{-\Lambda}\,\phi_{ll'}^{\Lambda}\,Y_{l\Lambda}\rangle . \tag{8}$$

Note that $V_{dkl'}^{\Lambda} = V_{dkl'}^{-\Lambda}$ because both terms on the r.h.s. of Eq. (5) must be of $\Sigma_u^+$ symmetry and the azimuthal parts of the target and continuum wave functions must cancel [3].

There is one more simplification introduced in Eq. (5) and it is omission of a sum over the target states $w(\tau)$ accounting for the correlation and polarization effects between the ejected electron and the neutral molecule. Such a sum would slightly change the definition of $V_{dkl'}^{\Lambda}$ since the sum would appear in the ket on the r.h.s of Eq. (8). Moreover, this sum would also enable the theory for the autodetachment decay into multiple final electronic states. However, these excited $^3\Pi_u$ states do not contribute into the present study and thus they are omitted for clarity.

The $V_{d\boldsymbol{k}'}$ term in (6) and (7) is a component of the level-shift operator $F(E)$ in Eq. (4) and it depends on the momentum vector $\boldsymbol{k}'$ expressed in the body frame of reference. Transformation to the unprimed coordinates attached to the laboratory frame is easily done through the Wigner D–functions as

$$V_{d\boldsymbol{k}} = \frac{1}{\sqrt{2}}\sum_{l'm}\left[V_{dkl'}^{\Lambda}D_{-\Lambda m}^{l'}(\hat{\boldsymbol{R}}) + \eta V_{dkl'}^{-\Lambda}D_{\Lambda m}^{l'}(\hat{\boldsymbol{R}})\right]Y_{l'm}^*(\hat{\boldsymbol{k}}) , \tag{9}$$

where the unit vector $\hat{\boldsymbol{R}}$ stands for the Euler angles of the diatomic molecule's orientation in the laboratory frame, i.e. $\hat{\boldsymbol{R}} \equiv (0,\theta,\phi)$.

The second term in the integral on the r.h.s of Eq. (4) represents the nuclear propagator

$$\langle\boldsymbol{k}^{(+)}|G_p|\boldsymbol{q}^{(+)}\rangle = \langle\boldsymbol{k}^{(+)}|(E-q^2/2-T-V_0(R)+i\epsilon)^{-1}|\boldsymbol{q}^{(+)}\rangle = \langle\boldsymbol{k}^{(+)}|G_0(E-q^2/2)|\boldsymbol{q}^{(+)}\rangle , \tag{10}$$

where $V_0(R)$ is the adiabatic potential energy curve of the neutral molecule in degenerate states $w_\Lambda$, $w_{-\Lambda}$, and $G_0$ is the Green's function of the neutral molecule [2, 7]. This Green's function can be expanded in the rovibrational eigenfunctions

$$Z_{\nu'N'M'}^{\Lambda\eta'}(\tau,\boldsymbol{R}) = \frac{1}{R}\chi_{\nu'N'}(R)X_{N'M'}^{\Lambda\eta'}(\tau,\hat{\boldsymbol{R}}) , \tag{11}$$

where the rotational wave function of the neutral molecule, in the non-$\Sigma$ electronic state, can be written as follows [6]:

$$X_{N'M'}^{\Lambda\eta'}(\tau,\hat{\boldsymbol{R}}) = \left(\frac{2N'+1}{8\pi}\right)^{1/2}\left[w_\Lambda(\tau)D_{\Lambda M'}^{N'}(\hat{\boldsymbol{R}}) + \eta' w_{-\Lambda}(\tau)D_{-\Lambda M'}^{N'}(\hat{\boldsymbol{R}})\right] . \tag{12}$$

Similar to anion case in Eq. (5) the symbol $\eta'$ represent the $(x'z')$-plane-reflection parity for the final neutral molecule. The expansion into the rotational states

$$G_0^{\Lambda\eta'}(E,\boldsymbol{R},\boldsymbol{R}') = \sum_{N'M'} X^{\Lambda\eta'}_{N'M'}(\hat{\boldsymbol{R}})\frac{1}{R}G_{0N'}(E,R,R')\frac{1}{R'}X^{*\Lambda\eta'}_{N'M'}(\hat{\boldsymbol{R}}') \;, \tag{13}$$

is then followed by the expansion of the radial Green's function into the vibrational states

$$G_{0N'}(E,R,R') = \sum_{\nu'} \frac{\chi_{\nu'}(R)\chi_{\nu'}(R')}{E - E_{\nu'N'} + i\epsilon} \;. \tag{14}$$

The energy levels $E_{\nu'N'}$ are rovibrational energies of the neutral system.

All the ingredients are now prepared to evaluate the angular matrix elements of the level-shift operator $F(E)$ defined by Eq. (4), i.e.

$$\langle Y_{N_1M_1}|F(E)|Y_{N_2M_2}\rangle = \frac{1}{RR'}\delta_{N_1N_2}\delta_{M_1M_2}f_{N_1}(E,R,R') \;, \tag{15}$$

where the radial component of the level-shift operator is defined as

$$f_N(E,R,R') = \sum_{lN'}\frac{1}{2}\left[1+\eta'(-1)^{l+N'+N}\right](2N'+1)\begin{pmatrix} l & N' & N \\ \Lambda & -\Lambda & 0\end{pmatrix}^2 \times \int \mathrm{d}k\, k\, V^{\Lambda}_{dkl}(R)G_{0N'}(E-k^2/2,R,R')V^{*\Lambda}_{dkl}(R') \;. \tag{16}$$

The remaining steps just follow Refs. [2, 5]. The integration over the momentum in Eq. (16) can be done analytically because of the resolvent form (14) of $G_{0N'}$. The level-shift operator is by this integration split into the real and imaginary components:

$$f_N(E,R,R') = \sum_{lN'}\frac{1}{2}\left[1+\eta'(-1)^{l+N'+N}\right](2N'+1)\begin{pmatrix} l & N' & N \\ \Lambda & -\Lambda & 0\end{pmatrix}^2 \times \sum_{\nu'}\chi_{\nu'N'}(R)\left[\Delta_l(E-E_{\nu'N'},R,R') - \frac{i}{2}\Gamma_l(E-E_{\nu'N'},R,R')\right]\chi_{\nu'N'}(R') \;, \tag{17}$$

where

$$\Gamma_l(\varepsilon,R,R') = 2\pi\, V^{\Lambda}_{dkl}(R)\, V^{*\Lambda}_{dkl}(R') \;, \tag{18}$$

$$\Delta_l(\varepsilon,R,R') = \frac{1}{2\pi}\mathcal{P}\int \mathrm{d}\varepsilon' \frac{\Gamma_l(\varepsilon',R,R')}{\varepsilon-\varepsilon'} \;. \tag{19}$$

While the expressions (16) and (17) are very similar to the ones derived in Ref. [2], the factor $g^{\eta'}_{lN'N} = (1+\eta'(-1)^{l+N'+N})/2$ is new for the case $\Lambda \neq 0$. In order to understand this two-valued factor (0 or 1), we first note that due to the bosonic nuclear spin statistics of the present $C_2^-$ system, only the odd rotational quanta $N$ of the decaying anion are populated. Furthermore, in the studied process the $\Sigma_u$ anion decays into the $\Pi_u$ neutral molecule and hence the continuum electron must be of the $\Pi_g$ symmetry, which contains only the even quanta of the ejected electron's angular momenta $l$. Finally, each of the final neutral rotational levels $N'$ is nearly doubly degenerate, split by the $\Lambda$-doubling effect. One of the states in this pair is symmetric and the other is antisymmetric with respect to the nuclear exchange. The upper and the lower components are distinguished by by the sign of $\eta'$ [3]. Therefore the factor $g$ simply selects only those final rotational states of

the neutral molecule, that are compatible with the nuclear spin conservation during the AD decay process.

The spherical symmetry of the level-shift operator $F(E)$ demonstrated by Eq. (15) suggests that, in the present model, different initial rotational levels $N$ are not coupled. However, every one of these initial levels can decay into those final states (each represented by the rotational quantum $N'$ of the neutral molecule and ejected electron's angular momentum $l$) that are allowed in the sum on the r.h.s. of Eq. (17). Furthermore, it is clear that the AD decay lifetimes into the final states are controlled by the partial widths $\Gamma_l$.

## II. LOCAL APPROXIMATION AND THE PARTIAL WIDTHS $\Gamma_l$

The localization of the nonlocal operator $F(E,R,R')$ is a commonly used technique [2, 5, 7, 8] exploiting different timescales of the electronic and nuclear motions. The interaction and the centrifugal terms of the radial Schrödinger equation are written as

$$\frac{N(N+1)}{2\mu R^2} + V_\mathrm{d}(R) + f_N(R) = \frac{N(N+1)}{2\mu R^2} + V_N^\mathrm{loc}(R) - \frac{i}{2}\Gamma_N^\mathrm{loc}(R)\ , \tag{20}$$

where

$$V_N^\mathrm{loc}(R) = V_0(R) + E_N^\mathrm{res}(R) = V_\mathrm{d}(R) + \Delta_N(E_N^\mathrm{res}(R), R, R)\ , \tag{21}$$

$$\Gamma_N^\mathrm{loc}(R) = \Gamma_N(E_N^\mathrm{res}(R), R, R)\ . \tag{22}$$

In the present study we neglect the $N$-dependence of the resonance energy $E^\mathrm{res}$ as the resonance is dominantly localized in a single partial wave $l = 2$. In this case the term $\Delta_l$ can be taken out of the sums in Eq. (17) and what remains, in the real part of $f_N$, is the resolution of identity. We estimate the error in the $V^\mathrm{loc}$ caused by this assumption in order of a few meV in the present study. Such a simplification will not be done for the imaginary part of the radial level-shift operator, because we want to explore the decay lifetimes over many orders of magnitude. Therefore, the $\Gamma_N^\mathrm{loc}$ remains as

$$\Gamma_N^\mathrm{loc}(R) = \sum_{lN'\nu'} g_{lN'N}^{\eta'}(2N'+1)\begin{pmatrix} l & N' & N \\ \Lambda & -\Lambda & 0 \end{pmatrix}^2 \Gamma_l^\mathrm{loc}(R)\,|\chi_{\nu'N'}(R)|^2\ . \tag{23}$$

Because the crossing point between the anion's and neutral curve depends on both rotational quantum numbers $N$ and $N'$, it would be very difficult to construct the $R$-dependent width function $\Gamma_l^\mathrm{loc}(R)$. Instead, we opt to replace the $R$-parameterized version of the local approximation by the energy parameterization, i.e.

$$\Gamma_l^\mathrm{loc}(E^\mathrm{res}) = \Gamma_l(E^\mathrm{res}, R(E^\mathrm{res}), R(E^\mathrm{res}))\ . \tag{24}$$

Such parameterization has been previous used to characterize the two-dimensional resonant surface of the $CF_3Cl$ molecule [9].

The partial widths were obtained at the neutral equilibrium geometry by calculations of the energy-dependent $K$ matrices with the diatomic UK R-matrix package [10]. An example of the eigenphases, one of the ingredients to determine the partial widths, is shown in the left panel of Fig. 1. The figure demonstrates that the resonant state is strongly localized in a single eigenphase channel that should not be mistaken for the angular momentum channel. This single eigenphase channel still consists of several partial waves with a dominant $d$-wave contribution. The technique for extraction of the partial widths was adopted from [11, 12]. The background $S$ matrix $S^0$ first diagonalized

$$\underline{U}^+\underline{S}^0\underline{U} = e^{2i\underline{\delta}^0}\ , \tag{25}$$

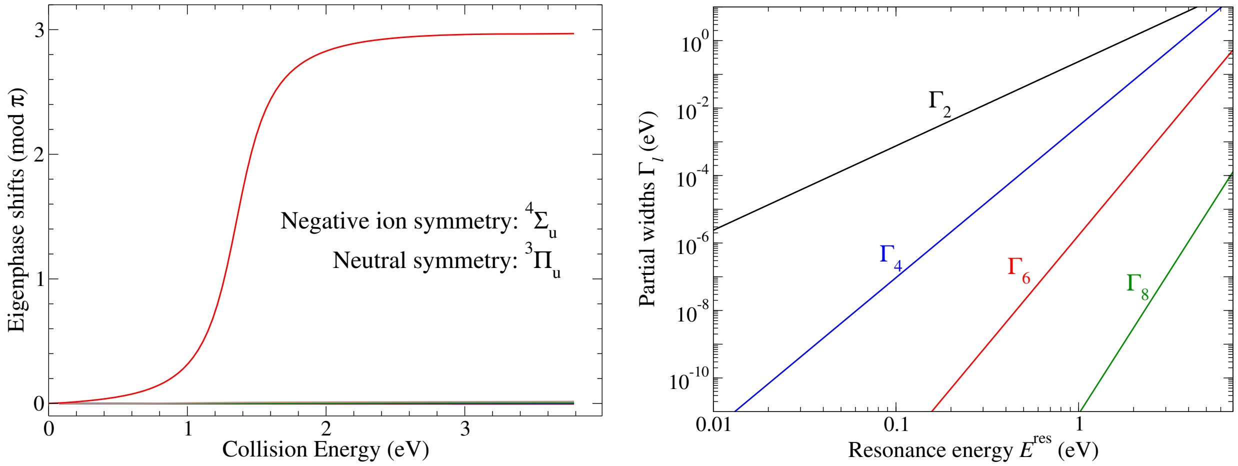


FIG. 1. Left panel: Eigenphases in the $^4\Sigma_u$ symmetry as functions of the collision energy. The nuclei are fixed at the equilibrium distance $R_0 = 2.49$ bohrs. Right panel: The energy dependence of the partial widths $\Gamma_l^{\rm loc}(E^{\rm res})$.

where $\underline{\delta}^0$ is the diagonal matrix of the background eigenphases $\delta^0_\alpha$. According to Macek [13], the partial widths can be obtained by fitting the energy dependence of the eigenphases

$$2(E - E^{\rm res}) = \sum_\alpha \Gamma_\alpha \cot\left[\delta^0_\alpha - \delta_\beta(E)\right] \tag{26}$$

for every eigenphase $\delta_\beta(E)$. The symbol $E^{\rm res}$ denotes the resonance energy and $\Gamma_\alpha$ describe partial widths of the decay into the eigenchannels of the background $S$ matrix $S^0$. However, our LCP model requires partial widths $\Gamma_l$ describing decays into the different partial waves of the continuum electron.

The partial widths $\Gamma_l$ can be obtained once the full $S$ matrix is transformed into the background eigenchannels as

$$\underline{U}\,\underline{A}\,\underline{U}^+ = \underline{S}. \tag{27}$$

While the matrix $\underline{A}$ is diagonal for $\underline{S}^0$, it contains rank-1 additional resonant term for the full matrix $\underline{S}$ [13]:

$$A_{\alpha\beta} = e^{i\delta^0_\alpha}\left[\delta_{\alpha\beta} - i\frac{(\Gamma_\alpha\Gamma_\beta)^{1/2}}{E - E^{\rm res} + i\Gamma/2}\right]e^{i\delta^0_\beta}\ . \tag{28}$$

This leads directly to

$$\Gamma_l^{1/2} = \sum_\alpha U_{l\alpha}\Gamma_\alpha^{1/2}\ , \tag{29}$$

where $U_{l\alpha}$ are the eigenvectors of the background $S$ matrix $S^0$ in Eq. (27) and the eigenchannel partial widths $\Gamma_\alpha$ are obtained by fitting the formula (26).

The partial widths from the equilibrium geometry, and from the corresponding resonant energy $E^{\rm res}(R_{\rm eq})$, were then extrapolated to other geometries by an application of the threshold law $\Gamma_l(\varepsilon) \sim \varepsilon^{l+1/2}$ [5]. The resulting energy dependence of the partial widths is shown in he right panel of Fig. 1.

While the resonant part of the anion curve was described in the previous section, the neutral and anion bound-state curves were obtained by the internally contracted Multi-Reference Configuration Interaction (MRCI) as implemented in MOLPRO 12 package of quantum-chemistry programs [14]. The wavefunctions for the MRCI method were generated by the state-averaged Multi-Configuration Self-Consistent Field (MCSCF) method with the active space of 8 and 9 electrons in 8 orbitals for $C_2$ and $C_2^-$, respectively. Molecular orbibrals were described by the Dunning's augmented correlation-consistent basis of quadruple-zeta quality aug-cc-pVQZ [15]. The energies of the $A^3\Pi_u$ neutral and

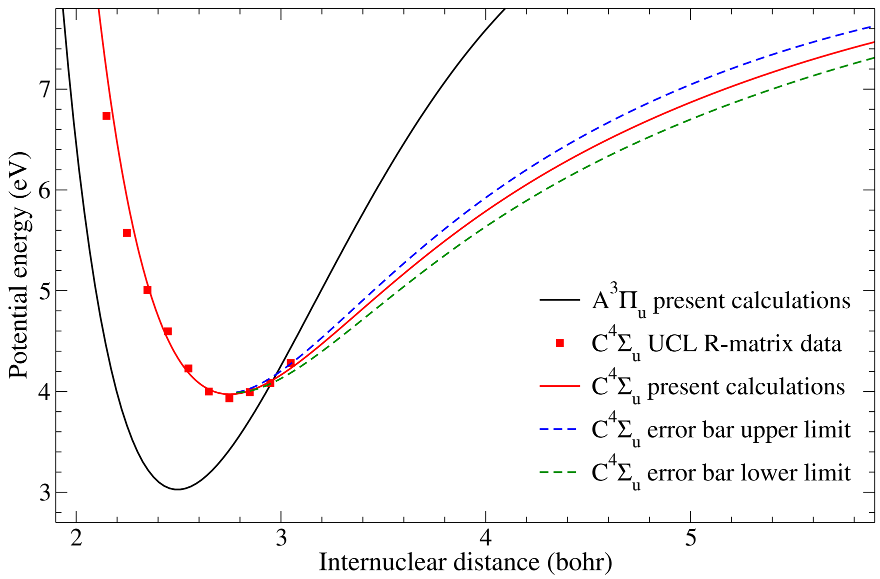


FIG. 2. Potential curves for the relevant neutral and anion states. The present calculations are shown with the full curves. Previous $R$-matrix calculations [16, 17] are displayed with squares. The dashed lines represent our estimate of the error bars for the present anion curve calculations.

$C^4\Sigma_u^+$ anion states, resulted from the present calculations, are displayed as the full curves in Fig. 2. These data together with the energy-dependent partial widths, shown in the right panel of Fig. 1, constitute all the electronic structure information necessary to build the effective Hamiltonian $H_{\rm eff}$ in Eq. (1) in the local complex approximation.

It is worth to note, that the present quartet anion curve was already studied previously by Halmová *et al.* [16, 17]. While the partial widths $\Gamma_l$ were not analyzed in Refs. [16, 17], the resonance energy $E^{\rm res}$ agrees reasonably well with the present calculations (see Fig. 2). However, the major discrepancy lies in the total resonance width $\Gamma$. Halmová [17] reports $\Gamma(R_{\rm eq}) = 0.28$ eV, while in the present calculations $\Gamma(R_{\rm eq}) = 0.48$ eV.

Finally, in order to estimate an impact of the accuracy of our *ab initio* calculations on the final results, we introduce computational error bars in form of upper- and lower-limit anion curves as shown in Fig. 2 by the dashed lines. These curves reach maximum deviations ±170 meV from the unperturbed $C^4\Sigma_{\rm u}$ curve at $R = 5$ bohrs. The value of the deviation is chosen arbitrarily, as our estimate for the typical error in the correlation energy for $\pi$-bonded systems described by the MRCI method.

[1] M. Čížek, J. Horáček, and W. Domcke, Phys. Rev. A **75**, 012507 (2007).

[2] M. Čížek and K. Houfek, in *Low-energy electron scattering from molecules, biomolecules and surfaces*, edited by P. Čársky and R. Čurík (CRC Press, Boca Raton, 2012) 1st ed., Chap. 4, pp. 91–125.
[3] G. Herzberg, *Molecular Spectra and Molecular Structure I. Spectra of Diatomic Molecules* (D. Van Nostrand Company, Inc., New York, 1950).
[4] T. F. O'Malley, Phys. Rev. **150**, 14 (1966).
[5] W. Domcke, Phys. Rep. **208**, 97 (1991).
[6] E. S. Chang and U. Fano, Phys. Rev. A **6**, 173 (1972).
[7] R. J. Bieniek, Phys. Rev. A **18**, 392 (1978).
[8] D. J. Haxton, C. W. McCurdy, and T. N. Rescigno, Phys. Rev. A **75**, 012710 (2007).
[9] M. Tarana, P. Wielgus, S. Roszak, and I. I. Fabrikant, Phys. Rev. A **79**, 052712 (2009).
[10] L. A. Morgan, C. J. Gillan, J. Tennyson, and X. S. Chen, J. Phys. B: Atom. Molec. Phys. **30**, 4087 (1997).
[11] A. U. Hazi, Phys. Rev. A **19**, 920 (1979).
[12] D. J. Haxton, C. W. McCurdy, and T. N. Rescigno, Phys. Rev. A **73**, 062724 (2006).
[13] J. Macek, Phys. Rev. A **2**, 1101 (1970).
[14] H. J. Werner, P. J. Knowles, R. Lindh, F. R. Knizia, F. R. Manby, M. Schütz, and Others, MOLPRO, version 2012.1, a package of ab initio programs (2012).
[15] T. H. Dunning, J. Chem. Phys. **90**, 1007 (1989).
[16] G. Halmová, J. D. Gorfinkiel, and J. Tennyson, J. Phys. B: Atom. Molec. Phys. **39**, 2849 (2006).
[17] G. Halmová, *R-matrix calculations of electron-molecule collisions with $C_2$ and $C_2^-$*, Ph.D. thesis, University College London (2008).
